# Supplementary material for: Drone Referring Localization: An Efficient Heterogeneous Spatial Feature Interaction Method For UAV Self-Localization
Source: arXiv:2208.06561 source file (2024-08-28)
Supplement: Supplementary file 1 [file appendix.pdf]

## APPENDIX A EFFECT OF POSITIVE SAMPLES

TABLE VI  
THE EFFECT OF THE POSITIVE SAMPLE SELECTION RANGE  $R$  ON MODEL PERFORMANCE.

| $R$ | RDS   |
|-----|-------|
| 1   | 57.21 |
| 2   | 56.67 |
| 3   | 55.72 |
| 5   | 52.19 |
| 7   | 47.76 |

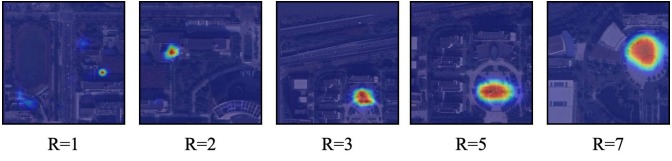

Fig. 13. The influence of different Center  $R$  on the distribution of heatmaps

To explore the effect of the distribution of positive samples on the FPI constructs. We test the effect of the distribution of positive samples on the model performance by different sampling ranges. The specific sampling procedure is described in Section III-E, and the visualized results are shown in Fig.5(B). We found that increasing the interval of positive samples has a negative impact on the performance of the model. We plotted the thermal distributions corresponding to different  $R$ , as shown in Fig.13. As  $R$  increases, the range of the thermal distribution increases, which is consistent with our intuition that this blurring of the thermal distribution makes the model less discriminative. We also try to attenuate the weights for the adjacent positive samples, however, the effect is still less than expected.

## APPENDIX B TRAIN AND TEST SET COMPOSITION

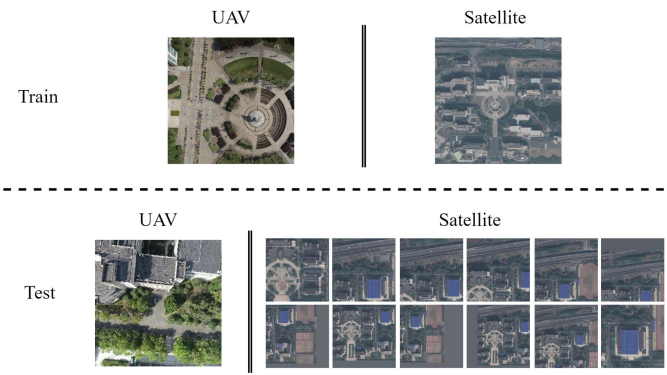

Fig. 14. Train and test set composition. The UAV and satellite map images in the training set are in a one-to-one relationship, and the data enhancement is done by random crop. The ratio of UAV and satellite images in the test set is 1:12

Fig. 14 enumerates the composition of the UAV and satellite images in the training and test sets. The center positions of the drone and satellite images in the training set are aligned. In the test set, the position of the UAV in the satellite image is randomly generated, and the real spatial scale corresponding to the satellite image is inconsistent.

## APPENDIX C FPI VS HUMAN

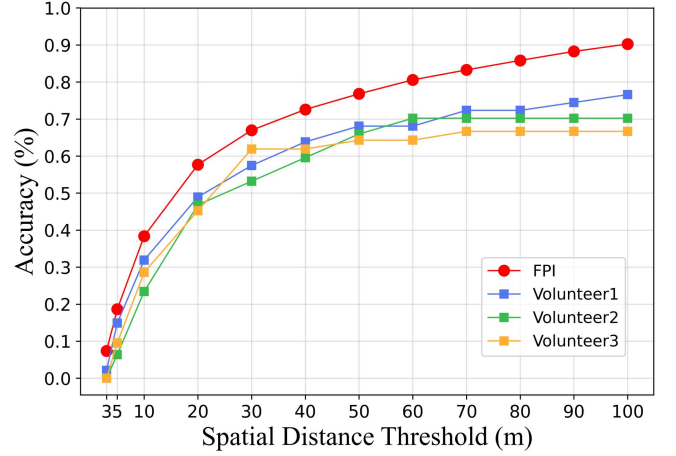

Fig. 15. Comparison of positioning accuracy of 3 volunteers and the FPI model

To demonstrate the superiority of the FPI architecture, we design an experiment that compares with the capabilities of the human eye. We recruited 3 volunteers for the experiment with a total duration of 30 minutes. The experiment provided volunteers with one set of drone and satellite images at a time. Volunteers figure out where the drone is in satellite imagery. The time limit for each set of data is 10s. If the person does not judge the result within 10s, it is regarded as a failed case and directly enters the next set of data. Before starting the formal experiment, volunteers had 30 minutes of training time to familiarize themselves with the positioning process. Finally, we use the MA to evaluate the positioning accuracy, and the experimental results are shown in Fig. 15. We can see that FPI has reached or even exceeded the ability of the human eye to locate. This also reflects the extremely challenging positioning task of multi-source data from another aspect.

## APPENDIX D

### DATASET COMPOSITION

TABLE VII  
STATISTICS ON THE NUMBER OF UNIVERSITY LISTS AND IMAGE PAIRS  
CONTAINED IN THE UL14 DATASET.

| #split | University Name                                                      | Pairs |
|--------|----------------------------------------------------------------------|-------|
| Train  | Zhejiang University of Finance & Economics                           | 600   |
|        | Zhejiang Gongshang University                                        | 600   |
|        | Hangzhou Vocational & Technical College                              | 600   |
|        | China Jiliang University                                             | 1374  |
|        | Zhejiang Police Vocational Academy                                   | 600   |
|        | Zhejiang Technical Institute of Economics                            | 600   |
|        | Zhejiang Institute of Economics and Trade                            | 894   |
|        | Zhejiang Normal University                                           | 600   |
|        | Zhejiang University of Water Resources and Electric Power            | 600   |
|        | China Jiliang University College of Modern Science<br>and Technology | 450   |
| Test   | Communication University of Zhejiang                                 | 600   |
|        | Hangzhou Dianzi University                                           | 531   |
|        | Zhejiang Financial College                                           | 600   |
|        | Zhejiang Sci-Tech University                                         | 600   |
